# Supplementary material for: Fate of a remnant solid disk around an eccentric giant planet
Source: arXiv:2407.11829 source file (2024-07-16)
Supplement: Supplementary file 1 [file appendix_decc.tex]

To keep other orbital elements unchanged, we put a velocity kick $\bf{v}_\mathrm{kick,p}$ at $\cos f_\mathrm{kick,p}$ which are given by: 
\begin{eqnarray}
    \bf{v}_\mathrm{kick,p} &=& (v_\mathrm{kick,p,R}, v_\mathrm{kick,p,T}, v_\mathrm{kick,p,Z}), \\
    \cos f_\mathrm{kick,p} &=& - \frac{2 e_\mathrm{p}}{1+{e_\mathrm{p}}^2},
\end{eqnarray}
with: 
\begin{eqnarray}
        v_\mathrm{kick,p,R} &=& -\frac{1 +e_\mathrm{p} \cos f_\mathrm{kick,p}}{e_\mathrm{p} \sin f_\mathrm{kick,p} \left(\cos E_\mathrm{p} -1/e_\mathrm{p} \right)} \sqrt{\frac{M_\mathrm{p}/M_\mathrm{s}}{a_\mathrm{p}(1-{e_\mathrm{p}}^2)}} \frac{1}{\tau_\mathrm{ecc}}, \\
        v_\mathrm{kick,p,T} &=& \frac{1}{\cos E_\mathrm{kick,p} -1/e_\mathrm{p}} \sqrt{\frac{M_\mathrm{p}/M_\mathrm{s}}{a_\mathrm{p}(1-{e_\mathrm{p}}^2)}} \frac{1}{\tau_\mathrm{ecc}}, \\
        v_\mathrm{kick,p,Z} &=& 0, \\
        \cos E_\mathrm{kick,p} &=& \frac{e_\mathrm{p}+\cos f_\mathrm{kick,p}}{1+e_\mathrm{p} \cos f_\mathrm{kick,p}}.
\end{eqnarray}
where $R$, $T$, and $Z$  are components in the cylindrical coordinate.
